# Supplementary material for: Towards efficient and accurate \emph{ab initio} solutions to periodic systems via transcorrelation and coupled cluster theory
Source: arXiv:2103.03176 source file (2021-03-04)
Supplement: Supplementary file 1 [file supp.pdf]

# Supplementary information for "Towards efficient and accurate *ab initio* solutions to periodic systems via transcorrelation and coupled cluster theory"

Ke Liao,[*] Thomas Schraivogel, Hongjun Luo, and Daniel Kats[†]
*Max Planck Institute for Solid State Research, Heisenbergstrasse 1, 70569 Stuttgart, Germany*

Ali Alavi[‡]
*Max Planck Institute for Solid State Research, Heisenbergstrasse 1, 70569 Stuttgart, Germany and Yusuf Hamied Department of Chemistry, University of Cambridge, Lensfield Road, Cambridge CB2 1EW, United Kingdom*

[*] ke.liao.whu@gmail.com
[†] d.kats@fkf.mpg.de
[‡] a.alavi@fkf.mpg.de

# I. INTERNAL CONTRACTIONS IN THE THREE-BODY INTEGRALS

The 3-body integrals can be written as an asymmetric form

$$\hat{W}_3 = -\frac{1}{2\Omega^2}\sum_{\sigma\sigma'\sigma''}\sum_{\mathbf{k}\mathbf{k}'\mathbf{r}\mathbf{s}\mathbf{t}} \tilde{u}(\mathbf{k}')\tilde{u}(\mathbf{k})\mathbf{k}'\cdot\mathbf{k}a^{\dagger}_{\mathbf{r}-\mathbf{k},\sigma}a^{\dagger}_{\mathbf{s}+\mathbf{k}',\sigma'}a^{\dagger}_{\mathbf{t}+\mathbf{k}-\mathbf{k}',\sigma''}a_{\mathbf{t},\sigma''}a_{\mathbf{s},\sigma'}a_{\mathbf{r},\sigma}, \tag{1}$$

where the indices are defined in the main text and conservation of momentum is used. In the following subsections, we will show the specific mathematical expressions for all contractions. The expressions are derived by using the Goldstone diagrams (not shown).

## A. Single contractions

There are 4 types of different single contractions, which are

$$\begin{aligned}
\hat{W}_3^{S1} &= -\frac{N_e}{2\Omega^2}\sum_{\sigma\sigma'}\sum_{\mathbf{krs}}(\tilde{u}(\mathbf{k}))^2k^2\{a^{\dagger}_{\mathbf{r}-\mathbf{k},\sigma}a^{\dagger}_{\mathbf{s}+\mathbf{k},\sigma'}a_{\mathbf{s},\sigma'}a_{\mathbf{r},\sigma}\},\\
\hat{W}_3^{S2} &= +\frac{1}{\Omega}\sum_{\sigma\sigma'}\sum_{\mathbf{krs}}\{a^{\dagger}_{\mathbf{r}-\mathbf{k},\sigma}a^{\dagger}_{\mathbf{s}+\mathbf{k},\sigma'}a_{\mathbf{s},\sigma'}a_{\mathbf{r},\sigma}\}\left(\frac{1}{\Omega}\sum_{\mathbf{i}}(\mathbf{i}-\mathbf{r}+\mathbf{k})\cdot\mathbf{k}\tilde{u}(\mathbf{k})\tilde{u}(\mathbf{i}-\mathbf{r}+\mathbf{k})\right),\\
\hat{W}_3^{S3} &= +\frac{1}{\Omega}\sum_{\sigma\sigma'}\sum_{\mathbf{krs}}\{a^{\dagger}_{\mathbf{r}-\mathbf{k},\sigma}a^{\dagger}_{\mathbf{s}+\mathbf{k},\sigma'}a_{\mathbf{s},\sigma'}a_{\mathbf{r},\sigma}\}\left(\frac{1}{\Omega}\sum_{\mathbf{i}}(\mathbf{r}-\mathbf{i})\cdot\mathbf{k}\tilde{u}(\mathbf{k})\tilde{u}(\mathbf{r}-\mathbf{i})\right),\\
\hat{W}_3^{S4} &= +\frac{1}{\Omega}\sum_{\sigma\sigma'}\sum_{\mathbf{krs}}\{a^{\dagger}_{\mathbf{r}-\mathbf{k},\sigma}a^{\dagger}_{\mathbf{s}+\mathbf{k},\sigma'}a_{\mathbf{s},\sigma'}a_{\mathbf{r},\sigma}\}\left(\frac{1}{\Omega}\sum_{\mathbf{i}}(\mathbf{r}-\mathbf{i}-\mathbf{k})\cdot(\mathbf{r}-\mathbf{i})\tilde{u}(\mathbf{r}-\mathbf{i})\tilde{u}(\mathbf{r}-\mathbf{i}-\mathbf{k})\right),
\end{aligned} \tag{2}$$

where the curly brackets refer to normal-ordering with respect to the reference determinant. Now we can define the $\tilde{\omega}^{rs}_{pq}$ by the following relation

$$\frac{1}{2}\sum_{\sigma\sigma''}\sum_{pqrs}\tilde{\omega}^{rs}_{pq}\{a^{\dagger}_{\mathbf{p},\sigma}a^{\dagger}_{\mathbf{q},\sigma'}a_{\mathbf{s},\sigma'}a_{\mathbf{r},\sigma}\} = \hat{W}_3^{S1}+\hat{W}_3^{S2}+\hat{W}_3^{S3}+\hat{W}_3^{S4}, \tag{3}$$

However, we notice that this effective 2-body integral is not symmetric with respect to the exchange of two electrons, due to the fact we used an asymmetric form of the 3-body integral. So we need to symmetrised it as follows

$$\tilde{\omega}^{rs}_{pq} \leftarrow \frac{1}{2}(\tilde{\omega}^{rs}_{pq}+\tilde{\omega}^{sr}_{qp}). \tag{4}$$

### B. Double contractions

The double contractions in the 3-body integrals result in the $\tilde{\omega}_p$ in the main text. It is a sum of 5 types of double contractions, which reads

$$\begin{aligned}
\tilde{\omega}_p = & \frac{N_e}{\Omega^2}\left(\sum_{\mathbf{i}} \tilde{u}^2(\mathbf{p}-\mathbf{i})(\mathbf{p}-\mathbf{i})^2\right) \\
& - \frac{1}{\Omega^2}\left(\sum_{\mathbf{ij}} (\mathbf{p}-\mathbf{i})\cdot(\mathbf{p}-\mathbf{j})\tilde{u}(\mathbf{p}-\mathbf{i})\tilde{u}(\mathbf{p}-\mathbf{j})\right) \\
& - \frac{1}{\Omega^2}\left(\sum_{\mathbf{ij}} (\mathbf{i}-\mathbf{j})\cdot(\mathbf{i}-\mathbf{p})\tilde{u}(\mathbf{i}-\mathbf{j})\tilde{u}(\mathbf{i}-\mathbf{p})\right) \\
& - \frac{1}{\Omega^2}\left(\sum_{\mathbf{ij}} (\mathbf{j}-\mathbf{i})\cdot(\mathbf{p}-\mathbf{i})\tilde{u}(\mathbf{j}-\mathbf{i})\tilde{u}(\mathbf{p}-\mathbf{i})\right) \\
& + \frac{1}{\Omega^2}\left(\sum_{\mathbf{ij}} (\mathbf{i}-\mathbf{j})^2\tilde{u}^2(\mathbf{i}-\mathbf{j})\right) .
\end{aligned} \tag{5}$$

### C. Triple contractions

There are 2 types of triple contractions which contribute to $E_{\mathrm{T}}$ mentioned in the main text:

$$E_{\mathrm{T}} = \frac{N_e}{2\Omega^2}\sum_{\sigma}\sum_{\mathbf{ij}} \tilde{u}^2(\mathbf{i}-\mathbf{j})(\mathbf{i}-\mathbf{j})^2 - \frac{1}{\Omega}\sum_{\sigma}\sum_{\mathbf{ij}}\left(\frac{1}{\Omega}\sum_{\mathbf{k}}(\mathbf{i}-\mathbf{k})\cdot(\mathbf{i}-\mathbf{j})\tilde{u}(\mathbf{i}-\mathbf{j})\tilde{u}(\mathbf{i}-\mathbf{k})\right) \tag{6}$$
